# Supplementary material for: CoinSeg: Contrast Inter- and Intra- Class Representations for Incremental Segmentation
Source: arXiv:2310.06368 source file (2023-10-10)
Supplement: Supplementary file 1 [file appendix.tex]

% 在swin-B介绍中提供模型参数地址
\tableofcontents
\vspace{6mm}

% \section{Erratum of Table 1 in the main paper}
% We apologise that part of the numerical results in Table 1 in the main paper was wrongly input by mistake (duplicated with the values above in method MicroSeg with ResNet101 as backbone). The correct values should be the highlighted (in \textcolor{red}{red}) ones in Table~\ref{tab:corrected}.
% \input{a_tables/A_corrected}
\section{More Experimental Details}
\subsection{Overlapped \& disjoint setup}
We provide a detailed explanation of the \textit{overlapped} and \textit{disjoint} settings in this section. The overlapped setting allows pixels in the samples from the sub-dataset $\bm{\mathcal{D}}^t$ to belong to any classes, including past classes from learning step 1 to $t-1$~(\ie, $\bm{\mathcal{C}}^{1:t-1}$), current classes~($\bm{\mathcal{C}}^t$), and future classes. However, only the classes in $\bm{\mathcal{C}}^t$ are annotated in $\bm y^t$. Moreover, images that contain multiple classes may appear in several learning steps with varying annotations. In contrast, the disjoint setting studied in prior works, such as ~\cite{MiB, SDR, RCIL}, comprises a non-overlapping subset of datasets. Each learning step contains a unique $\bm{\mathcal{C}}^t$, and its pixels only belong to classes seen in $\bm{\mathcal{C}}^{1:t-1}$ or $\bm{\mathcal{C}}^t$. Notably, the overlapped setup is more realistic as it imposes a weaker restriction on the data than the disjoint setup.

\subsection{Reproducibility}
In all experiments, CoinSeg adopts the same mask proposals and the number of proposals $N=100$, according to prior practice as in the class incremental semantic segmentation~(CISS) method MicroSeg~\cite{MicroSeg}. 
We adopt the official \href{https://github.com/SwinTransformer/storage/releases/tag/v1.0.0}{\textcolor{orange}{\texttt{Pre-trained Model}}} of Swin Transformer~\cite{swintransformer} for all experimental results. 
In the case of CoinSeg-M, which is CoinSeg equipped with a memory sampling strategy, we implemented the strategy using the official code of the prior CISS work SSUL~\cite{SSUL}. To be more specific, the strategy is based on random sampling from the training dataset, while also ensuring that at least one sample of every seen class is present in the memory bank. 
% Please refer to the attached code for more information about reproducibility.

\section{Additional Experimental Analysis}

\subsection{Detailed experimental results of CoinSeg}

%------------------------------------------------------------------------------------
\begin{table*}[h]
  \centering
  \caption{Detailed experimental results of CoinSeg over each class.}
  \begin{adjustbox}{max width=\linewidth}
\begin{tabular}{c|ccccccccccc}
\toprule
\multirow{4}{*}{\textbf{VOC 10-1}} & bg & aero & bike & bird & boat & bottle & bus & car & cat & chair & cow \\ \cline{2-12} 
 & 88.0 & 89.9 & 40.8 & 94.1 & 76.3 & 88.5 & 91.1 & 89.7 & 96.2 & 48.4 & 77.2 \\ 
 \cline{2-12} 
 &  {table} &  {dog} &  {horse} &  {mbike} &  {person} &  {plant} &  {sheep} &  {sofa} &  {train} & \multicolumn{1}{c}{TV} &  {\textbf{mIoU}} \\ \cline{2-12} 
 & 37.8 & 89.4 & 75.3 & 83.7 & 85.5 & 47.1 & 59.5 & 27.4 & 74.8 & 53.2 & \textbf{72.5}  \\ 
 \midrule
\multirow{4}{*}{\textbf{VOC 15-1}} & bg & aero & bike & bird & boat & bottle & bus & car & cat & chair & cow \\ \cline{2-12} 
 & 90.3 & 89.8 & 43.5 & 95.2 & 79.3 & 88.0 & 91.2 & 90.8 & 96.3 & 47.1 & 78.1 \\ \cline{2-12} 
 &  {table} &  {dog} &  {horse} &  {mbike} &  {person} &  {plant} &  {sheep} &  {sofa} &  {train} & \multicolumn{1}{c}{TV} &  {\textbf{mIoU}} \\ \cline{2-12} 
 & 68.5 & 93.3 & 91.0 & 92.0 & 89.7 & 43.7 & 64.1 & 27.0 & 72.7 & 55.4 & \textbf{75.5} \\ 
 \midrule
\multirow{4}{*}{\textbf{VOC 19-1}} & bg & aero & bike & bird & boat & bottle & bus & car & cat & chair & cow \\ \cline{2-12} 
 & 93.9  & 91.8  & 43.0 & 94.5 & 76.4 & 87.2 & 95.0 & 89.6 & 96.5 & 49.1 & 91.5 \\ 
 \cline{2-12} 
 &  {table} &  {dog} &  {horse} &  {mbike} &  {person} &  {plant} &  {sheep} &  {sofa} &  {train} & \multicolumn{1}{c}{TV} &  {\textbf{mIoU}} \\ \cline{2-12} 
 & 65.9 & 89.7 & 90.1 & 90.3 & 90.9 & 63.0 & 93.0 & 54.0 & 86.0 & 44.8 & \textbf{79.8} \\ 
 \midrule
\multirow{4}{*}{\textbf{VOC 15-5}} & bg & aero & bike & bird & boat & bottle & bus & car & cat & chair & cow \\ \cline{2-12} 
 & 91.3 & 90.9 & 43.8 & 95.4 & 74.5 & 85.2 & 90.0 & 91.3 & 95.2 & 49.1 & 79.5 \\ \cline{2-12} 
 &  {table} &  {dog} &  {horse} &  {mbike} &  {person} &  {plant} &  {sheep} &  {sofa} &  {train} & \multicolumn{1}{c}{TV} &  {\textbf{mIoU}} \\ \cline{2-12} 
 & 66.7 & 90.5 & 91.0 & 90.9 & 90.1 & 55.2 & 72.4 & 31.3 & 84.0 & 73.1 & \textbf{77.6} \\ 
 \midrule
 % 2-2
\multicolumn{1}{c|}{\multirow{4}{*}{\textbf{VOC 2-2}}} & bg & aero & bike & bird & boat & bottle & bus & car & cat & chair & cow \\ \cline{2-12} 
\multicolumn{1}{l|}{} & 89.1 & 85.4 & 35.8 & 53.2 & 56.9 & 76.7 & 88.5 & 80.3 & 88.0 & 18.3 & 64.4 \\ \cline{2-12} 
\multicolumn{1}{l|}{} &  {table} &  {dog} &  {horse} &  {mbike} &  {person} &  {plant} &  {sheep} &  {sofa} &  {train} & \multicolumn{1}{c}{TV} &  {\textbf{mIoU}} \\ \cline{2-12} 
\multicolumn{1}{l|}{} & 43.0 & 59.2 & 64.9 & 79.8 & 80.8 & 60.2 & 51.8 & 32.4 & 74.1 & 67.9 & \textbf{64.3} \\ 
\bottomrule
\end{tabular}
  \end{adjustbox}
  \label{tab:voc_class}
\end{table*}
Tab.~\ref{tab:voc_class} shows the detailed experimental results over each class in the Pascal VOC 2012~\cite{VOC_everingham2010pascal} dataset.

\subsection{CoinSeg with ResNet101 backbone}
\begin{table*}[t!]
  \centering
\caption{
    Comparison with state-of-the-art methods on Pascal VOC 2012 with ResNet101. \textcolor{lightgray}{Joint} is the upperbound.
  }
  \label{tab:resnet}
  \begin{adjustbox}{max width=\linewidth}
  \begin{tabular}{l|c|ccc|ccc|ccc|ccc|ccc}
\toprule
\multirow{2}{*}{Method} & \multirow{2}{*}{Backbone} & \multicolumn{3}{c|}{\textbf{VOC 10-1 (11 steps)}} & \multicolumn{3}{c|}{\textbf{VOC 15-1 (6 steps)}} & \multicolumn{3}{c|}{\textbf{VOC 19-1 (2 steps)}} & \multicolumn{3}{c|}{\textbf{VOC 15-5 (2 steps)}} & \multicolumn{3}{c}{\textbf{VOC 2-2 (10 steps)}} \\
 &  & 0-10 & 11-20 & all & 0-15 & 16-20 & all & 0-19 & 20 & all & 0-15 & 16-20 & all & 0-2 & 3-20 & all \\ \midrule
\textcolor{lightgray}{Joint} & \textcolor{lightgray}{ResNet101} & \textcolor{lightgray}{82.1}  & \textcolor{lightgray}{79.6} & \textcolor{lightgray}{80.9} & \textcolor{lightgray}{82.7} & \textcolor{lightgray}{75.0} & \textcolor{lightgray}{80.9} & \textcolor{lightgray}{81.0} & \textcolor{lightgray}{79.1} & \textcolor{lightgray}{80.9} & \textcolor{lightgray}{82.7} & \textcolor{lightgray}{75.0} & \textcolor{lightgray}{80.9} & \textcolor{lightgray}{76.5} & \textcolor{lightgray}{81.6} & \textcolor{lightgray}{80.9} \\
LwF-MC~\cite{LwF_li2017learning} & ResNet101 & 4.7 & 5.9 & 4.9 & 6.4 & 8.4 & 6.9 & 64.4 & 13.3 & 61.9 & 58.1 & 35.0 & 52.3 & 3.5 & 4.7 & 4.5\\
ILT~\cite{ILT_michieli2019incremental} & ResNet101 & 7.2 & 3.7 & 5.5 & 8.8 & 8.0 & 8.6 & 67.8 & 10.9 & 65.1 & 67.1 & 39.2 & 60.5 & 5.8 & 5.0 & 5.1 \\
MiB~\cite{MiB} & ResNet101 & 12.3 & 13.1 & 12.7 & 34.2 & 13.5 & 29.3 & 71.4 & 23.6 & 69.2 & 76.4 & 50.0 & 70.1 & 41.1 & 23.4 & 25.9 \\
SDR~\cite{SDR} & ResNet101 & 32.1 & 17.0 & 24.9 & 44.7 & 21.8 & 39.2 & 69.1 & 32.6 & 67.4 & 57.4 & 52.6 & 69.9 & 13.0 & 5.1 & 6.2 \\
PLOP~\cite{PLOP} & ResNet101 & 44.0 & 15.5 & 30.5 & 65.1 & 21.1 & 54.6 & 75.4 & 37.4 & 73.5 & 75.7 & 51.7 & 70.1 & 24.1 & 11.9 & 13.7 \\
RCIL~\cite{RCIL} & ResNet101 & 55.4 & 15.1 & 34.3 & 70.6 & 23.7 & 59.4 & 68.5 & 12.1 & 65.8 & 78.8 & 52.0 & 72.4 & 28.3 & 19.0 & 19.4 \\
SSUL~\cite{SSUL} & ResNet101 & 71.3 & 46.0 & 59.3 & 77.3 & 36.6 & 67.6 & 77.7 & 29.7 & 75.4 & 77.8 & 50.1 & 71.2 & 62.4 & 42.5 & 45.3 \\
SSUL-M\cite{SSUL} & ResNet101 & 74.0 & 53.2 & 64.1 & 78.4 & 49.0 & 71.4 & 77.8 & 49.8 & 76.5 & 78.4 & 55.8 & 73.0 & 58.8 & 45.8 & 47.6 \\
MicroSeg~\cite{MicroSeg} & ResNet101 & 72.6 & 48.7 & 61.2 & 80.1 & 36.8 & 69.8 & 78.8 & 14.0 & 75.7 & 80.4 & 52.8 & 73.8 & 61.4 & 40.6 & 43.5 \\
MicroSeg-M~\cite{MicroSeg} & ResNet101 & \textbf{77.2} & 57.2 & \textbf{67.7} & 81.3 & 52.5 & 74.4 & 79.3 & 62.9 & 78.5 & \textbf{82.0} & 59.2 & \textbf{76.6} & 60.0 & 50.9 & 52.2 \\ 
\midrule
CoinSeg~(Ours) & ResNet101 & 73.7 & 45.0 & 60.1 & 80.6 & 36.2 & 70.1 & \textbf{80.7} & 29.4 & 78.3 & 80.8 & 31.0 & 68.9 & 68.3 & 46.2 & 49.4 \\
CoinSeg-M~(Ours) & ResNet101 & 71.1 & \textbf{60.2} & 65.9 & \textbf{81.5} & \textbf{54.0} & \textbf{75.0} & 80.3 & \textbf{44.8} & \textbf{78.6} & 81.3 & \textbf{61.3} & \textbf{76.6} & \textbf{66.7} & \textbf{53.9} & \textbf{55.7} \\

\bottomrule
\end{tabular}
  \end{adjustbox}
\end{table*}

To further validate the effectiveness of our proposed approach and ensure a fair comparison with other methods from a different perspective, we conducted additional experiments with the CoinSeg method using ResNet101 as the backbone. 
The results are presented in Tab.~\ref{tab:resnet}, From which we can see, even with a relatively weaker backbone, the results indicate that our approaches, including CoinSeg and CoinSeg-M, are still competitive, and achieve state-of-the-art performance across multiple incremental scenarios. 
%These results provide further evidence of the effectiveness of our approach.

\subsection{Experimental results of disjoint setting}

To provide a thorough comparison with prior works on CISS, we further present the experimental results of our proposed methods, CoinSeg and CoinSeg-M, in the disjoint setting in Tab.~\ref{tab:disjoint_all}. We evaluate our methods using both the ResNet101 and Swin-B backbones. The results show that our methods achieve state-of-the-art performance, surpassing prior works on CISS.

\begin{table*}[!htp]
\centering
\caption{
    Experimental results on Pascal VOC 2012 for \textit{disjoint} setup. \dag: CoinSeg with Swin-B backbone.
    % SSUL-M denotes the result using exemplar memory.
  }
  
  \begin{adjustbox}{max width=\linewidth}
\begin{tabular}{l|ccc|ccc|ccc} 
\toprule
\multirow{2}{*}{Method}                  & \multicolumn{3}{c|}{\textbf{VOC 15-1 (6 steps)}} & \multicolumn{3}{c|}{\textbf{VOC 19-1 (2 steps)}} & \multicolumn{3}{c}{\textbf{VOC 15-5 (2 steps)}}  \\
            & 0-15  & 16-20 & all                              & 0-19  & 20    & all                              & 0-15  & 16-20 & all                              \\ 
\midrule

LwF-MC~\cite{LwF_li2017learning}            & 4.5  & 7.0  & 5.2                             & 63.0 & 13.2 & 60.5                            & 67.2 & 41.2 & 60.7                            \\
ILT~\cite{ILT_michieli2019incremental}               & 3.7  & 5.7  & 4.2                             & 69.1 & 16.4 & 66.4                            & 63.2 & 39.5 & 57.3                            \\
MiB~\cite{MiB}               & 46.2 & 12.9 & 37.9                            & 69.6 & 25.6 & 67.4                            & 71.8 & 43.3 & 64.7                            \\
SDR~\cite{SDR} & 59.4 & 14.3 & 48.7 & 70.8 & 31.4 & 68.9 & 74.6 & 44.1 & 67.3 \\
PLOP~\cite{PLOP}              & 57.9 & 13.7 & 46.5                            & 75.4 & 38.9 & 73.6                            & 71.0 & 42.8 & 64.3                            \\
RCIL~\cite{SDR} & 66.1 & 18.2 & 54.7 & 68.9 & 15.0 & 66.3 & 75.0 & 42.8 & 67.3 \\
SSUL~\cite{SSUL}              & 74.0 & 32.2 & 64.0                            & 77.4 & 22.4 & 74.8                            & 76.4 & 45.6 & 69.1                            \\
SSUL-M~\cite{SSUL}            & 76.5 & 43.4 & 68.6                            & 77.6 & 43.9 & 76.0                            & 76.5 & 48.6 & 69.8                            \\ 

MicroSeg~\cite{MicroSeg}   & 73.7 & 24.1 & 61.9                            & 80.6 & 16.0 & 77.4                          & 77.4 & 43.4 & 69.3                            \\
MicroSeg-M~\cite{MicroSeg} & 80.0  & 47.6  & 72.3                            & 81.1  & 45.1  & 79.4                             & 80.7  & 55.2  & 74.7                             \\ 
CoinSeg~(Ours)   & 75.6 & 30.9 & 64.9                            & 80.5 & 25.1 & 77.9                    & 79.6 & 43.8 & 71.1                            \\
CoinSeg-M~(Ours) & 80.9  & 47.4  & 72.9                            & 80.8  & 50.6  & 79.4                             & 81.7 & 58.9  & 76.3                             \\ 
\midrule
CoinSeg\dag~(Ours)   & \textbf{82.0} & 46.1 & 73.4                            & 82.0 & 34.0 & 80.2                          & 82.1 & 55.3 & 75.7                            \\
CoinSeg-M\dag~(Ours) & \textbf{82.0}  & \textbf{49.6}  & \textbf{74.3}                             & \textbf{82.6}  & \textbf{66.3}  & \textbf{81.8}                             & \textbf{82.9} & \textbf{61.7}  & \textbf{77.9}                             \\ 
\bottomrule
\end{tabular}
  \end{adjustbox}
  \label{tab:disjoint_all}
\end{table*}

\subsection{Ablation study of contrast intra-class diversity}

As highlighted in the main paper, strategies aimed at contrasting intra-class diversity are critical for learning robust representations. 
In this regard, we provide quantitative evidence to support this claim. Specifically, Tab.~\ref{tab:abl_intra} reveals that using $\mathcal{L}_{int}$ only yields a marginal improvement in performance. 
This suggests that while assigning a representation to each class via average pooling may be effective to some extent, it is not the optimal strategy, and the improvement in performance is limited. 
On the other hand, combining $\mathcal{L}_{int}$ with $\mathcal{L}_{itr}$ leads to a significant improvement in overall performance. These findings indicate that contrastive learning of intra-class diversity is an effective approach for robust representation learning.

\subsection{Ablation to pseudo-labeling strategy in $\mathcal{L}_{int}$}
As detailed in the main paper Sec.~\textcolor{Mahogany}{3.2}, we employ pseudo-labeling within $\mathcal{L}_{int}$ to extract categories learned in previous learning steps. To illustrate its impact, we report the performance of $\mathcal{L}_{int}$ just with the current class labels in Tab.~\ref{tab:PL_Lint} Right (`GT' row). We can see that the proposed pseudo-labeling (PL) boosts the performance.
\begin{table}[h]
\centering
  \vspace{-2mm}
  \caption{
  % \textcolor[rgb]{0.01,0.01,0.15}{
     Ablations to pseudo-labeling  in $\mathcal{L}_{int}$. 
     GT: ground truth, PL: pseudo label.
  }
  \label{tab:PL_Lint}
  \begin{adjustbox}{max width=0.96\linewidth}
     \begin{tabular}{c|ccc}
      \toprule
    \multirow{2}{*}{label}     &\multicolumn{3}{c}{\textbf{VOC 15-1 (6 steps)}}      \\
 &   0-15          & 16-20         & all                \\ \midrule
              
 GT & 81.6  & 54.3   & 75.1        \\
                                                            
 PL & 82.7 & 52.5 & \textbf{75.5} \\

      \bottomrule
    \end{tabular}
  
  \end{adjustbox}
  \vspace{-2mm}
\end{table}

\begin{table}[t]
  \centering
  \caption{
     Ablation study of Contrast inter- \& intra- class representations, $\lambda_r$. All experiments are conducted on VOC 15-1.
  }
  \label{tab:abl_intra}
  \begin{adjustbox}{max width=\linewidth}
     \begin{tabular}{ccc|ccc}
      \toprule
      \multirow{2}{*}{{Method}} & \multirow{2}{*}{$\mathcal{L}_{int}$} &\multirow{2}{*}{$\mathcal{L}_{itr}$} & \multicolumn{3}{c}{\textbf{VOC 15-1 (6 steps)}}                                                                  \\
                          &                                     &  & 0-15          & 16-20         & all                   \\ \midrule
       \multirow{3}{*}{CoinSeg}                
                      & \xmark                                      & \xmark & 80.4  & 43.7   & 71.6          \\
                      & \cmark                                      & \xmark & 80.8  & 45.9   & 72.4~(+0.8)          \\
                      & \cmark                                      & \cmark & 82.7 & 52.5 & \textbf{75.5}~(+3.9) \\
      \bottomrule
    \end{tabular}
  
  \end{adjustbox}
  \vspace{-2mm}
\end{table}

\subsection{Discussions of adaption of Swin Transformer}

\begin{table*}[t]
  \centering
  \caption{
     Comparisons of CoinSeg with different backbones.  \dag: Re-implemented with Swin-B backbone.
  }
  \label{tab:cmpofbkbn}
  \begin{adjustbox}{max width=0.9\linewidth}
     \begin{tabular}{l|c|ccc|ccc|ccc|ccc|ccc}
\toprule
\multirow{2}{*}{Method} & \multirow{2}{*}{Backbone} & \multicolumn{3}{c|}{\textbf{VOC 10-1 (11 steps)}} & \multicolumn{3}{c|}{\textbf{VOC 15-1 (6 steps)}} & \multicolumn{3}{c|}{\textbf{VOC 19-1 (2 steps)}} & \multicolumn{3}{c|}{\textbf{VOC 15-5 (2 steps)}} & \multicolumn{3}{c}{\textbf{VOC 2-2 (10 steps)}} \\
 &  & 0-10 & 11-20 & all & 0-15 & 16-20 & all & 0-19 & 20 & all & 0-15 & 16-20 & all & 0-2 & 3-20 & all \\ \midrule

\methodname & Resnet101 & 73.7 & 45.0 & 60.1 & 80.6 & 36.2 & 70.1 & 80.7 & 29.4 & 78.3 & 80.8 & 31.0 & 68.9 & 68.3 & 46.2 & 49.4 \\
CoinSeg\dag & Swin-B & 80.0 & 63.4 & 72.5 & 82.7 & 52.5 & 75.5 & 81.5 & 44.8 & 79.8 & 82.1 & 63.2 & 77.6 & 70.1 & 63.3 & 64.3 \\  
\bottomrule
\end{tabular}
  
  \end{adjustbox}
  \vspace{-2mm}
\end{table*}

Our proposed contrast intra- and inter-class diversity representation approach places a greater emphasis on local information. 
In contrast to conventional CNN-based architectures, the Swin Transformer offers superior feature representation capabilities for local patches~\cite{han2022survey,swintransformer}. Hence, we choose the Swin Transformer as the backbone of the model. 
Tab.~\ref{tab:cmpofbkbn} show the comparison of both backbones, ResNet101 and Swin Transformer. 
The results show that CoinSeg achieves a significant improvement in performance with the Swin Transformer, particularly in more challenging long-term scenarios such as VOC 10-1 and 2-2.

Meanwhile, due to the freeze strategy, prior methods may not be able to fully take advantage of the backbone's performance. 
As a result, the performance improvement of prior methods is limited when replacing ResNet101 with Swin Transformer as the backbone. 
This conclusion can be drawn by comparing the experimental results presented in the main paper. 
However, our proposed CoinSeg method shows significant performance improvement when using Swin Transformer as the backbone.

It is important to note that while applying the Swin Transformer results in improved performance, our approach does not depend solely on a stronger backbone. As shown in Tab.~\ref{tab:resnet}, CoinSeg achieves state-of-the-art performance even when using the ResNet101 backbone.

\subsection{Search of hyper-parameters}
% lambda
% tau

Here we present the results of the hyper-parameters search, including $\lambda_r$, $\lambda_c$, $\lambda_{lr}$ and $\tau$. We have done the parameter search on five orders of magnitude on VOC 15-1, for $\lambda_r$  $\lambda_c$ and $\lambda_{lr}$. 
The results of Tab.~\ref{tab:abl_reg} show $\lambda_r$, the hyper-parameter to balance regularization constraints, is not sensitive to the choice of these parameters. Even if the $\lambda_r$ varies by several orders of magnitude~($10^{-3}$ to $1$), the performance is stable. The results show that our proposed method, CoinSeg, is effective over a wide range of choices of hyper-parameters. 
Tab.~\ref{tab:abl_con} presents the parameter search of $\lambda_c$, the hyper-parameter weight of contrast inter- and intra-class representations~(\textit{Coin}).
And Tab.~\ref{tab:abl_lr} is the performance comparison with different choices of $\lambda_{lr}$ in flexible initial learning rate.
Additionally, we also report the more detailed experimental results in different incremental scenario~(VOC 10-1) in Tab.~\ref{tab:abl_lr10-1}.
The results lead to similar conclusions.
Furthermore, we have done a parameter search for threshold $\tau$ for pseudo-label in Tab.~\ref{tab:abl_tau}. The conclusions are still similar. 

Additionally, we also conduct a hyperparametric search within a similar magnitude, as most previous works did, as shown in Tab.~\ref{tab:sameMagnitude}.
Our method shows a performance fluctuation of only 0.4\% in this perspective. 
This demonstrates the robustness of our proposed CoinSeg with respect to hyperparameters.
As a summary, we choose $\lambda_r=0.1$, $\lambda_c=0.01$, $\lambda_{lr}=10^{-3}$ and $\tau = 0.7$ for the best performance.

\subsection{Reproduction of past methods}
In this paper, a portion of the experimental results are obtained through reproducing previous methods, e.g., the performance of previous methods equipped with the Swin-B backbone. Note that we have made extensive efforts to optimize the performance of previous methods on the Swin transformer, to facilitate a fair comparison. Tab.~\ref{tab:choiceOfK} show the parameter tuning the most crucial hyperparameter, $K$, in previous method MicroSeg.

\section{More Qualitative Results}
\begin{figure*}[t]
\centering 
{\includegraphics[width=1.00\linewidth]{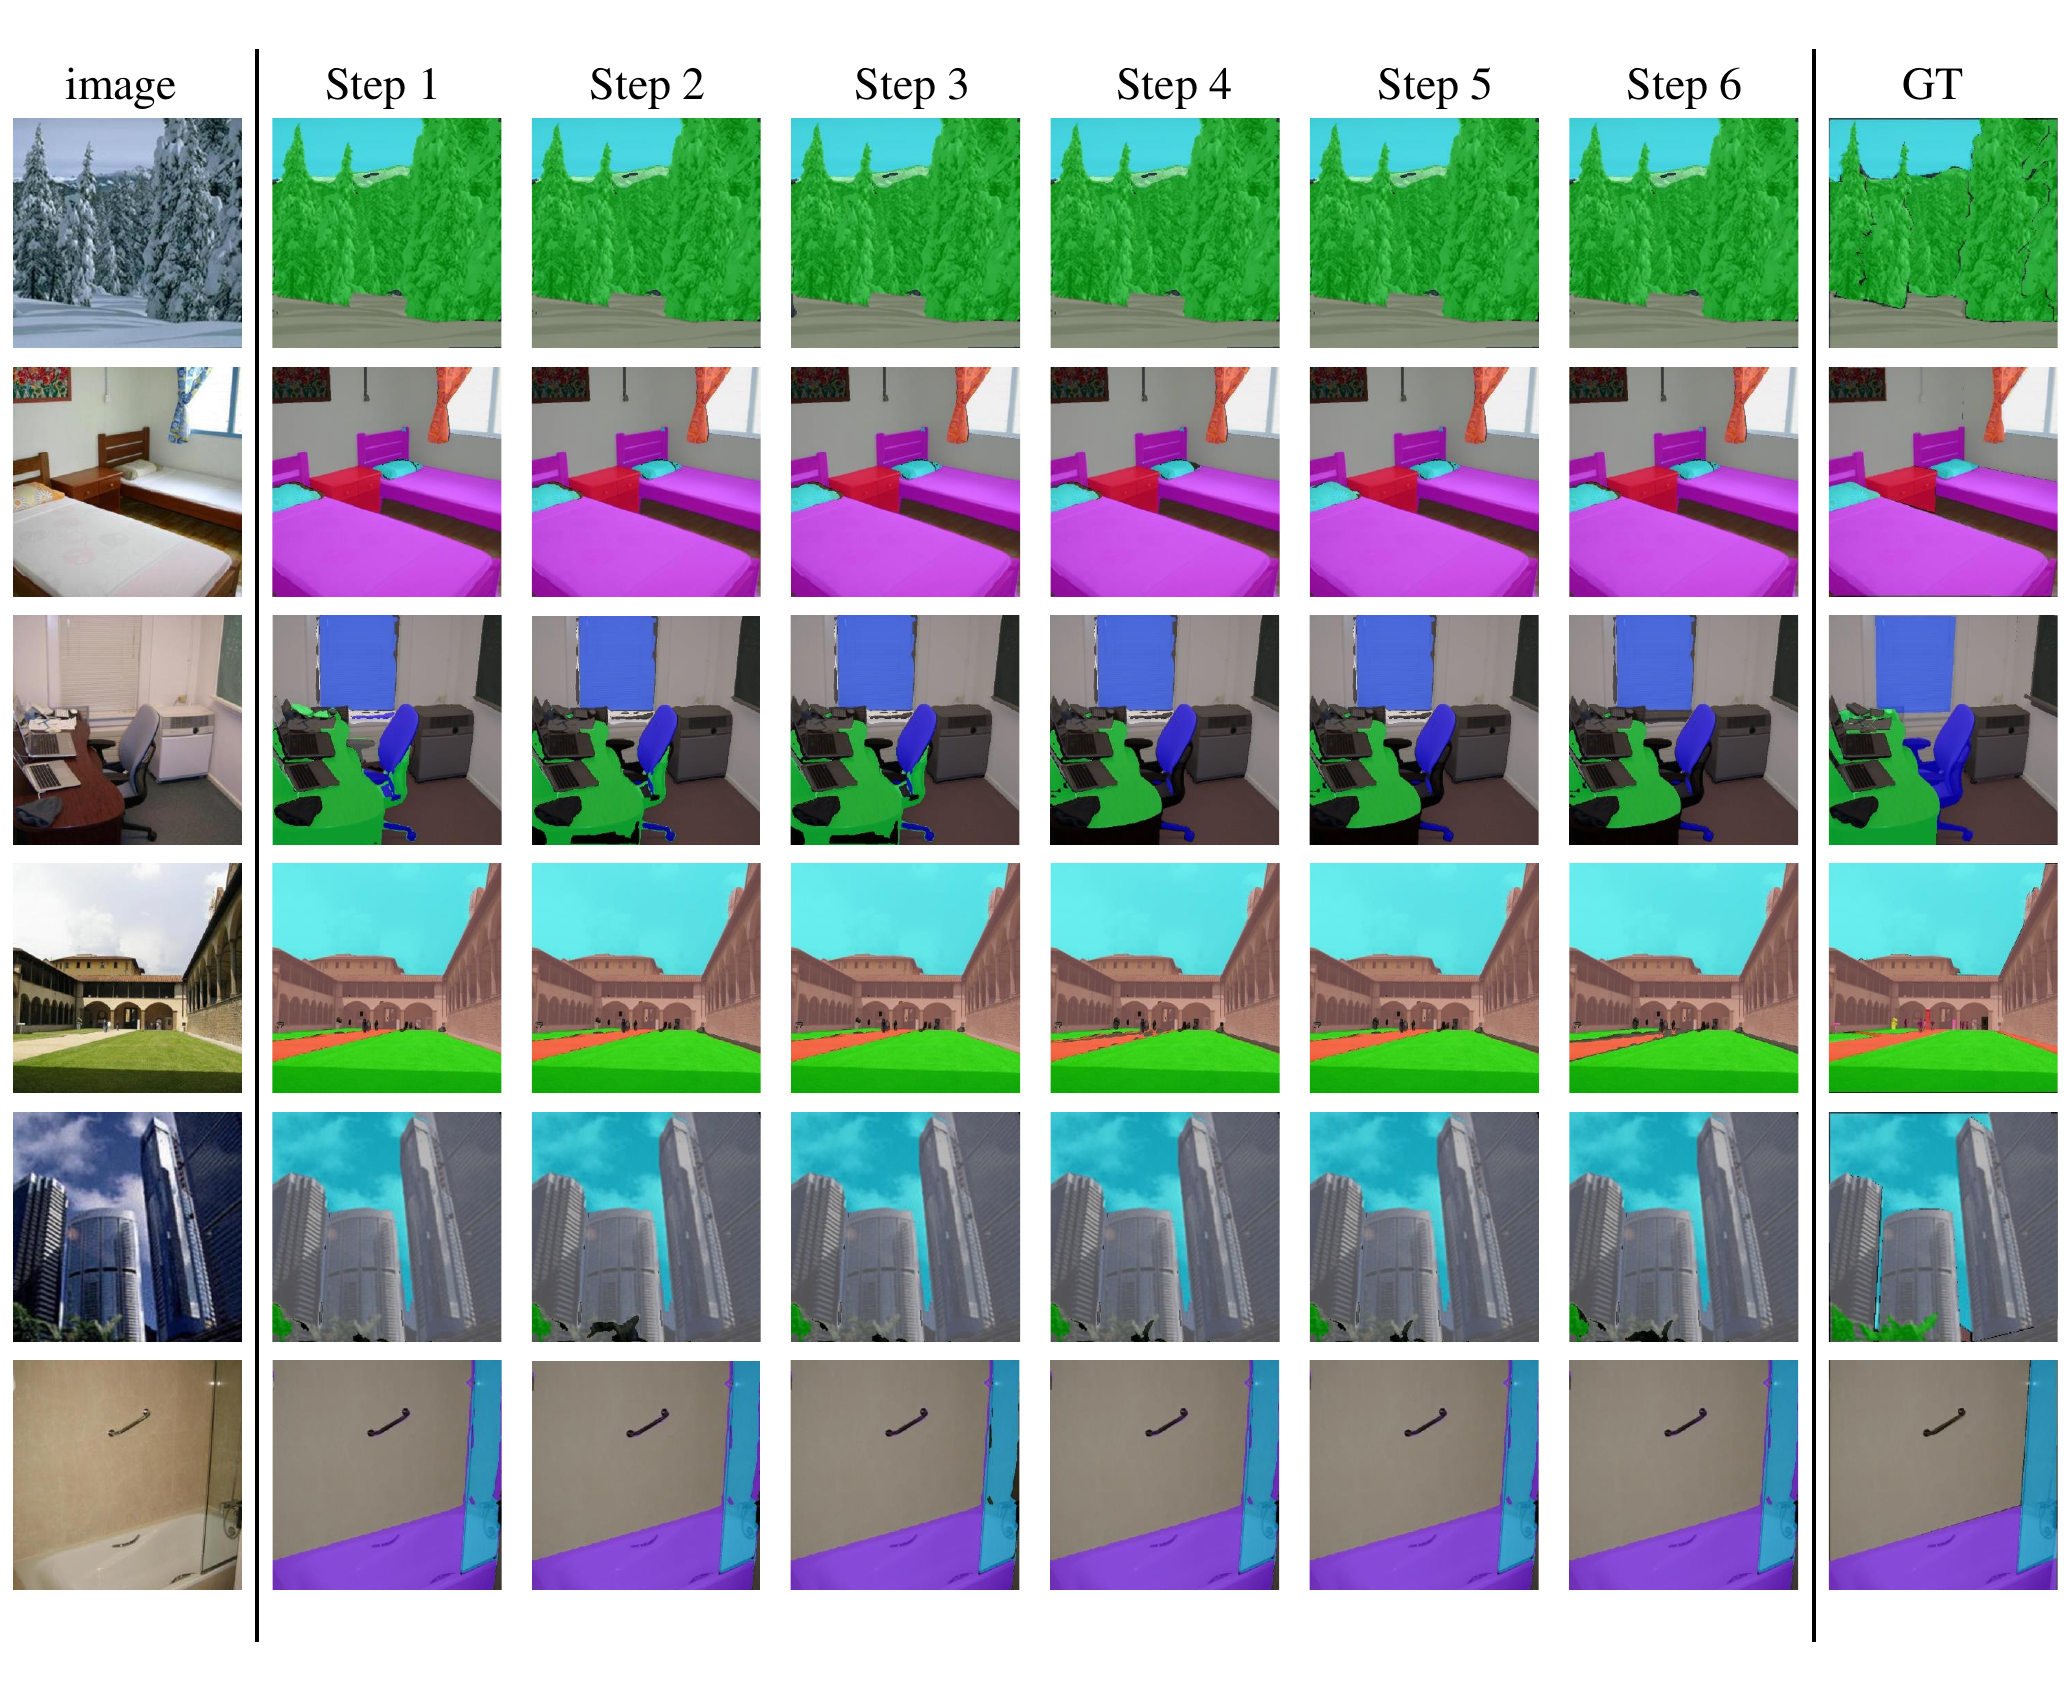}
}
\vspace{-8mm}
\caption{{Qualitative analysis for ADE 100-10.}}
% \vspace{-0.3cm}
\label{fig:quat_ade}
 \end{figure*}
In addition to the qualitative results shown in the main paper, here in Fig.~\ref{fig:quat_ade} shows more qualitative results of ADE20K~\cite{ADE_zhou2017scene} dataset. 
We conducted a long-term incremental scenario, ADE 100-10, consisting of six steps to better evaluate the effectiveness of CoinSeg. 
To provide a more comprehensive analysis, we present qualitative results of multiple scenes, including indoor and outdoor, things and stuff. 
The results show that CoinSeg rarely forgets old concepts during incremental learning steps, validating its effectiveness in long-term incremental scenarios.
\begin{table}[t]
  \centering
  \caption{
     Parameter search of hyper-parameter of regularization constraints, $\lambda_r$. All experiments are conducted on VOC 15-1.
    % SSUL-M denotes the result using exemplar memory.
  }
  \label{tab:abl_reg}
  \begin{adjustbox}{max width=\linewidth}
     \begin{tabular}{cc|ccc}
      \toprule
      \multirow{2}{*}{{Method}}  &\multirow{2}{*}{$\lambda_r$} & \multicolumn{3}{c}{\textbf{VOC 15-1 (6 steps)}}                                                                  \\
                          &                                       & 0-15          & 16-20         & all                   \\ \midrule
       \multirow{5}{*}{CoinSeg}                             
                                & $10^{-3}$ & 80.9          & 53.3          & 74.3                 \\
                                & $0.01$ &  81.9         & 52.6          & 74.9          \\
                                & $0.1$ & 82.7          & 52.5          & \textbf{75.5}          \\
                                & $1$ & 81.7 & 50.6 & 74.3 \\
                                & $10$ & 80.8 & 50.4 & 73.5 \\
      \bottomrule
    \end{tabular}
  
  \end{adjustbox}
  \vspace{-2mm}
\end{table}
\begin{table}[t]
  \centering
  \caption{
     Parameter search of hyper-parameter to balance \textit{Coin}, $\lambda_c$. All experiments are conducted on VOC 15-1.
}
  \label{tab:abl_con}
  \begin{adjustbox}{max width=\linewidth}
     \begin{tabular}{cc|ccc}
      \toprule
      \multirow{2}{*}{{Method}}  &\multirow{2}{*}{$\lambda_c$} & \multicolumn{3}{c}{\textbf{VOC 15-1 (6 steps)}}                                                                  \\
                          &                                       & 0-15          & 16-20         & all                   \\ \midrule
       \multirow{5}{*}{CoinSeg}                             
                        & $10^{-3}$ & 81.4          & 48.9          & 73.7                  \\
                        & $0.01$ & 82.7          & 52.5          & \textbf{75.5}          \\
                        & $0.1$ & 82.4          & 51.8          & 75.1          \\
                        & $1$ & 81.8 & 49.9 & 74.2 \\
                        & $10$ & 80.6 & 46.6 & 72.5 \\
      \bottomrule
    \end{tabular}
  
  \end{adjustbox}
  \vspace{-2mm}
\end{table}
\begin{table}[t]
  \centering
  \caption{
     Parameter search of hyper-parameter in flexible initial learning rate, $\lambda_{lr}$. All experiments are conducted on VOC 15-1.
    % SSUL-M denotes the result using exemplar memory.
  }
  \label{tab:abl_lr}
  \begin{adjustbox}{max width=\linewidth}
     \begin{tabular}{cc|ccc}
      \toprule
      \multirow{2}{*}{{Method}}  &\multirow{2}{*}{$\lambda_{lr}$} & \multicolumn{3}{c}{\textbf{VOC 15-1 (6 steps)}}                                                                  \\
                          &                                       & 0-15          & 16-20         & all                   \\ \midrule
       \multirow{5}{*}{CoinSeg}                             
                        & $10^{-4}$ & 83.0          & 48.4          & 74.5                  \\
                        & $10^{-3}$ & 82.7          & 52.5          & \textbf{75.5}          \\
                        & $0.01$ & 82.6          & 51.1          & 75.1          \\
                        & $0.1$ & 82.3 & 50.7 & 74.8 \\
                        & $1$ & 81.3 & 49.6 & 73.8 \\
      \bottomrule
    \end{tabular}
  
  \end{adjustbox}
  \vspace{-2mm}
\end{table}
\begin{table}[h]
  \centering

  \caption{
    More detailed hyperparameter search of $\lambda_{lr}$ on VOC 10-1, within similar magnitudes.
  }
  \label{tab:abl_lr10-1}
  \begin{adjustbox}{max width=\linewidth}
     \begin{tabular}{cc|ccc}
      \toprule
      \multirow{2}{*}{{Method}}  &\multirow{2}{*}{$\lambda_{lr}$} & \multicolumn{3}{c}{\textbf{VOC 10-1 (11 steps)}}                                                                  \\
                          &                                       & 0-10          & 11-20         & all                   \\ \midrule
       \multirow{3}{*}{CoinSeg}       
                        & $1 \times 10^{-4}$ & 80.4         & 58.6          &   69.9                \\
                        & $5 \times 10^{-4}$ & 80.2         & 59.1          &   70.2                \\
                        & $1\times10^{-3}$ & 80.1          & 60.0          & \textbf{70.5}          \\
                        & $2\times 10^{-3}$ & 79.8          & 59.5          &   70.1        \\
                        & $5\times 10^{-3}$ & 79.0          & 59.2          &   69.6        \\

      \bottomrule
    \end{tabular}
  
  \end{adjustbox}

\end{table}

\begin{table}[t]
  \centering
  \caption{
     Parameter search of hyper-parameter: threshold $\tau$ for pseudo-label. All experiments are conducted on VOC 15-1.
    % SSUL-M denotes the result using exemplar memory.
  }
  \label{tab:abl_tau}
  \begin{adjustbox}{max width=\linewidth}
     \begin{tabular}{cc|ccc}
      \toprule
      \multirow{2}{*}{{Method}}  &\multirow{2}{*}{$\tau$} & \multicolumn{3}{c}{\textbf{VOC 15-1 (6 steps)}}                                                                  \\
                          &                                       & 0-15          & 16-20         & all                   \\ \midrule
       \multirow{5}{*}{CoinSeg}                             & $0.1$ & 81.4          & 47.5          & 73.3                  \\
                                                            & $0.3$ &  81.3         & 49.7          & 73.8          \\
                                                            & $0.5$ & 82.0          & 50.6          & 74.5          \\
                                                            & $0.7$ & 82.7          & 52.5          & \textbf{75.5} \\
                                                            & $0.9$ & 81.1 & 51.9 & 74.1 \\
      \bottomrule
    \end{tabular}
  
  \end{adjustbox}
  \vspace{-2mm}
\end{table}
\begin{table}[h]
\color[rgb]{0,0,0.18} % 文字颜色
    \vspace{-2mm}
  \centering
  \caption{
     Hyperparameter search of $\lambda_c$ within a similar magnitude, in VOC 15-1.
  }
  \label{tab:sameMagnitude}
  \begin{adjustbox}{max width=0.96\linewidth}

    \begin{tabular}{c|ccc}
\toprule
\multirow{2}{*}{$\lambda_c$} & \multicolumn{3}{c}{VOC 15-1 (6 steps)} \\
 & 0-15 & 16-20 & all \\ \midrule
$0.75\times10^{-2}$ & 82.5 & 53.0 & 75.5(+0.0) \\
$1\times10^{-2}$ & 82.7 & 52.5 & \textbf{75.5} \\
$3\times10^{-2}$ & 82.7 & 52.3 & 75.4(-0.1) \\
$5\times10^{-2}$ & 82.6 & 51.4 & 75.1(-0.4) \\
$7\times10^{-2}$ & 82.6 & 52.0 & 75.2(-0.3) \\ \bottomrule
\end{tabular}
  
  \end{adjustbox}
  \vspace{-6mm}
\end{table}
\begin{table}[h]
\color[rgb]{0,0,0.18} 
    \vspace{-2mm}
  \centering
  \caption{
     Hyperparameter search of $K$ in MicroSeg with Swin-B backbone (Left), and $\lambda_c$ within a similar magnitude~(Right).
  }
  \label{tab:choiceOfK}
  \begin{adjustbox}{max width=0.96\linewidth}
     \begin{tabular}{c|ccc}
\toprule
\multirow{2}{*}{$K$} & \multicolumn{3}{c}{VOC 15-1 (6 steps)} \\
 & 0-15 & 16-20 & all \\ 
 \midrule
1 & 78.8 & 37.1 & 68.9 \\
3 & 79.1 & 38.6 & 69.5 \\
5 & 80.5 & 40.8 & \textbf{71.0} \\
7 & 81.4 & 35.9 & 70.6 \\
9 & 81.2 & 36.1 & 70.4 \\ 
\bottomrule
\end{tabular}
  
  \end{adjustbox}
  \vspace{-6mm}
\end{table}

In addition, we provide more qualitative results in Fig.~\ref{fig:quat_more} and Fig.~\ref{fig:quat_more2}, for VOC 15-1. 
In some samples, novel classes appear in the incremental steps, and the results demonstrate that our proposed CoinSeg can effectively adapt to these new categories. 
Meanwhile, in samples which only contians base classes, the predictions remain stable through all learning steps, which indicates CoinSeg alleviating forgetting.
\vspace{-2mm}

\newpage

\paragraph{Limitations, future work and social impact}

Although our approach, CoinSeg, achieves state-of-the-art performance in numerous benchmarks, forgetting still exists in long-term scenarios.
For future work, it might be interesting to explore how a well-designed deep learning model architecture can be better applied to tackle the long-term incremental learning tasks.

All of our experimental results are produced on public datasets and the research of CoinSeg has no obvious AI ethical issues, to the best of our knowledge. But training deep learning models does have some potential environmental impact due to the power consumption. We hope that our proposed approach can help researchers to conduct further exploration of class incremental semantic segmentation.

\begin{figure*}[t]
\centering 

{\includegraphics[width=0.95\linewidth]{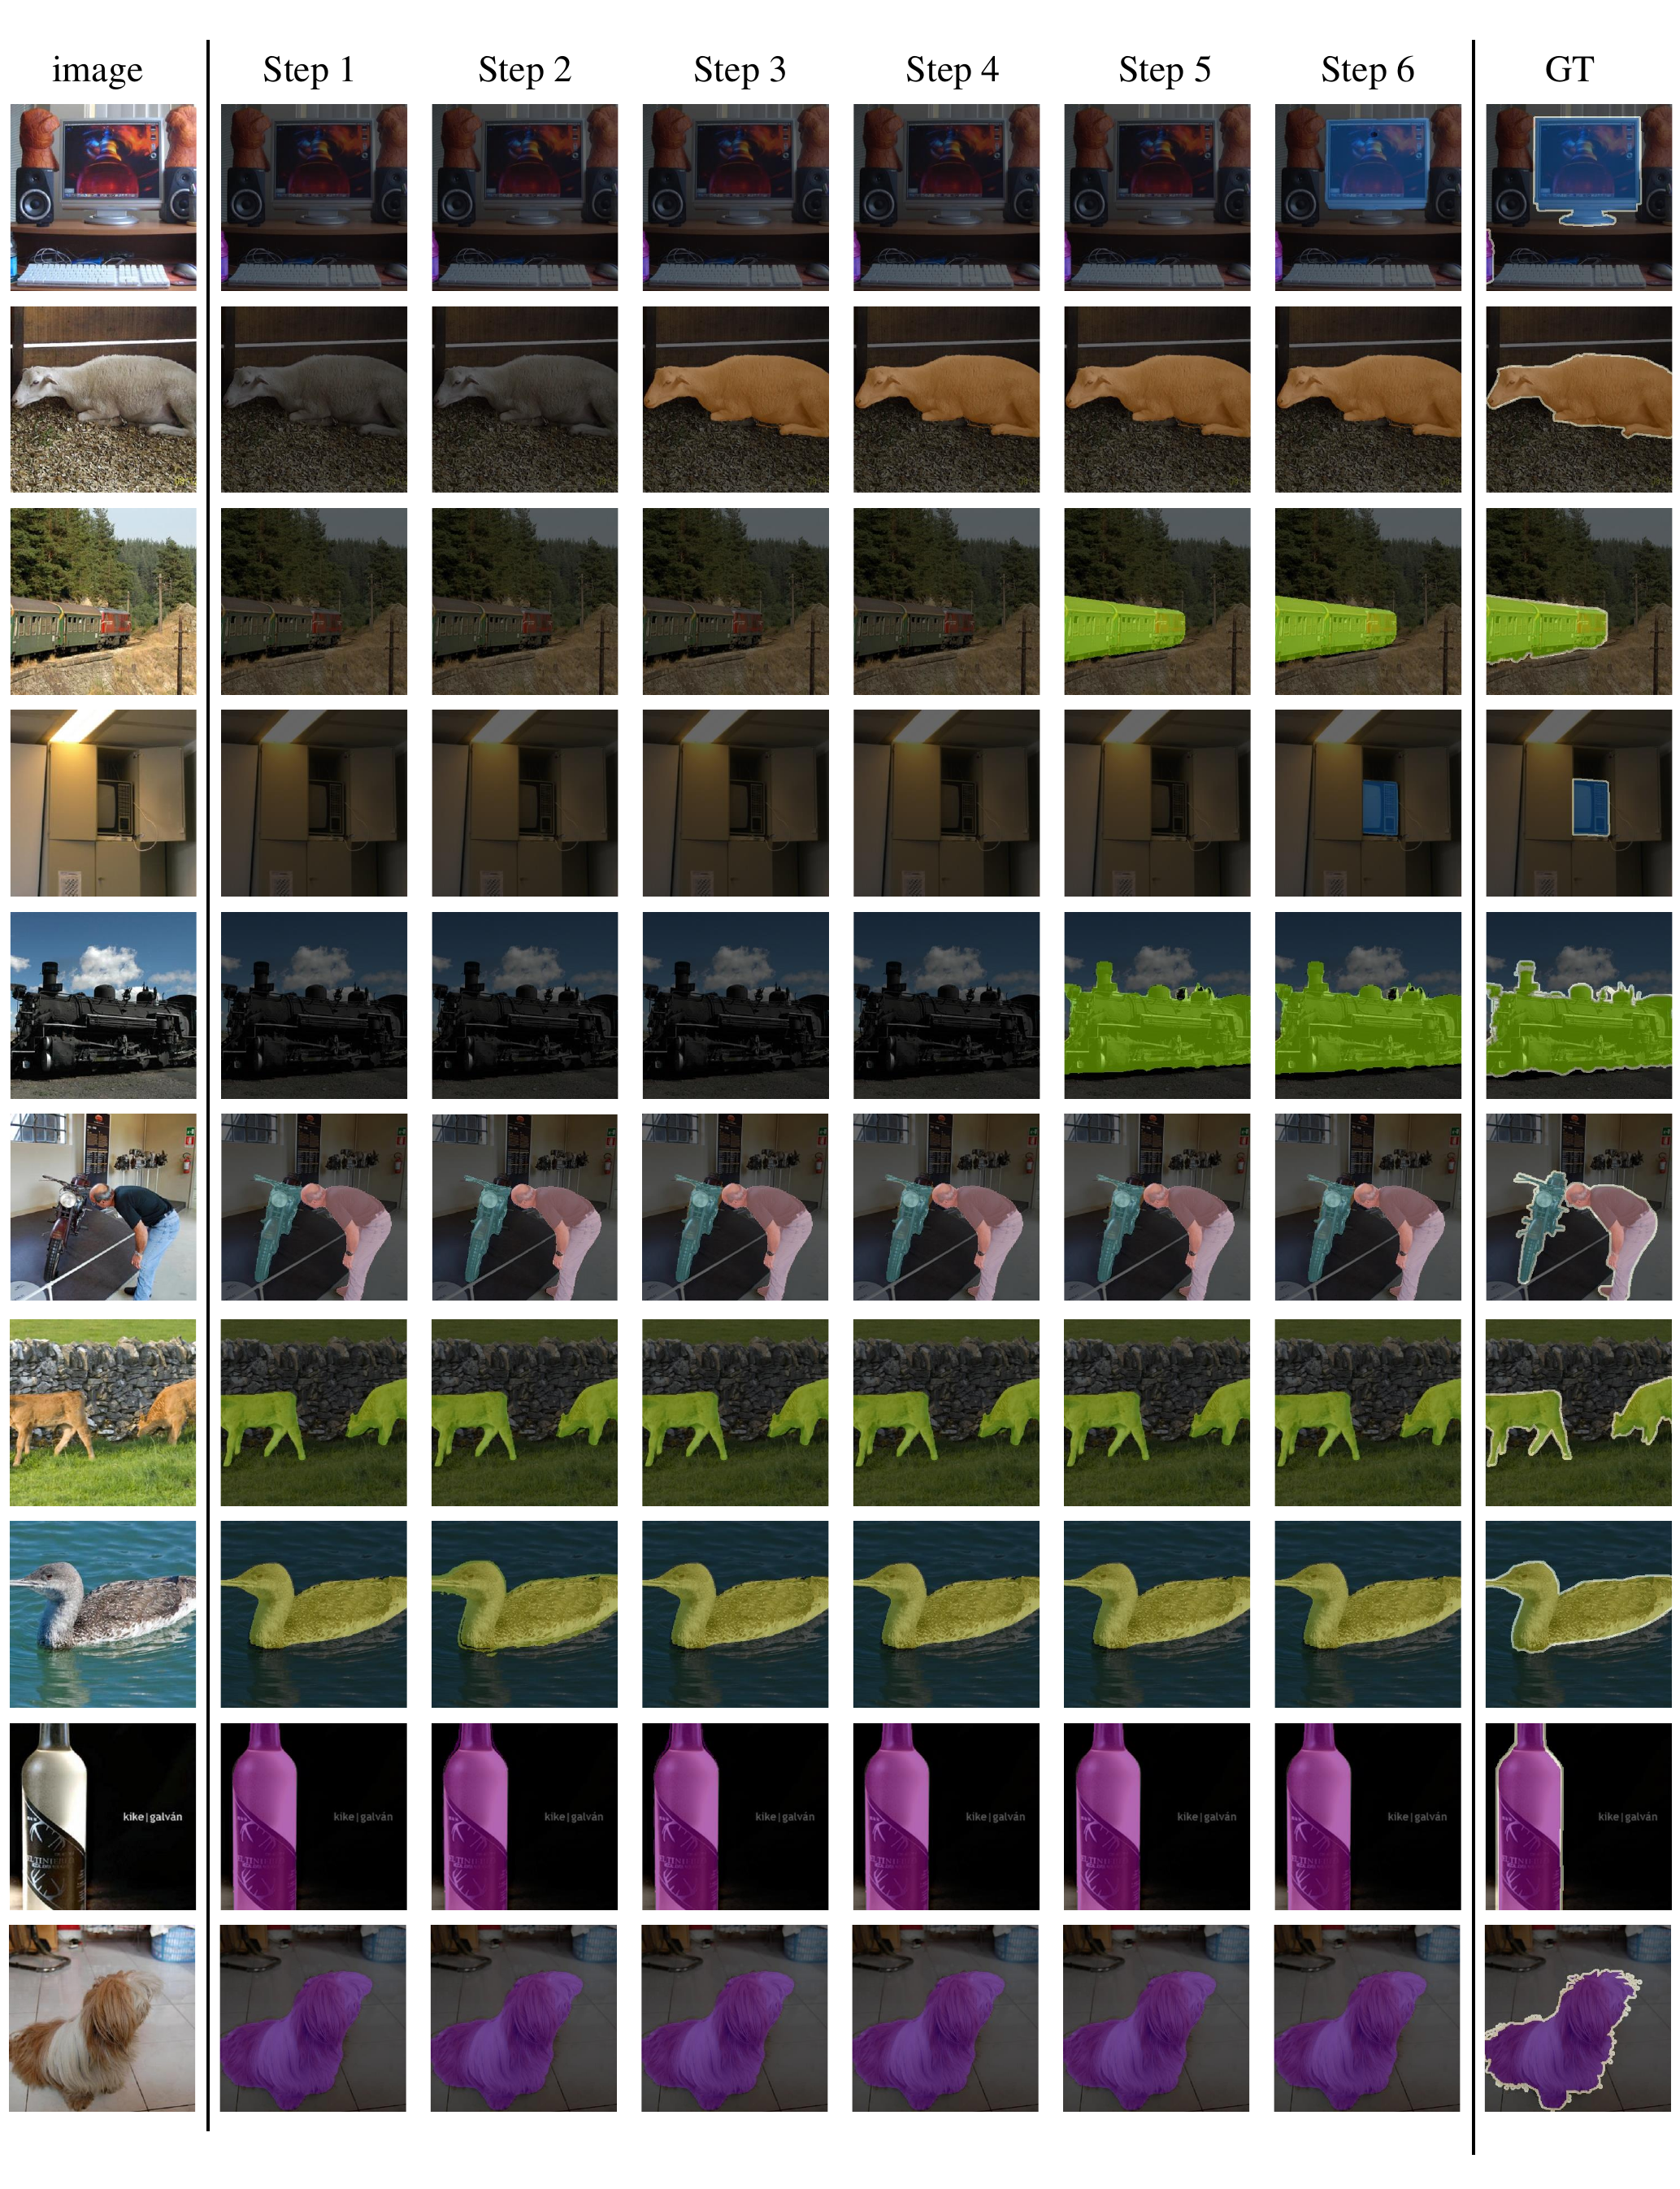}
}

\caption{{More qualitative analysis of CoinSeg. The white borderline is \textbf{ignore label} in Pascal VOC 2012 dataset.}}
% \vspace{-0.3cm}
\label{fig:quat_more}
 \end{figure*}
\begin{figure*}[t]
\centering 

{\includegraphics[width=0.95\linewidth]{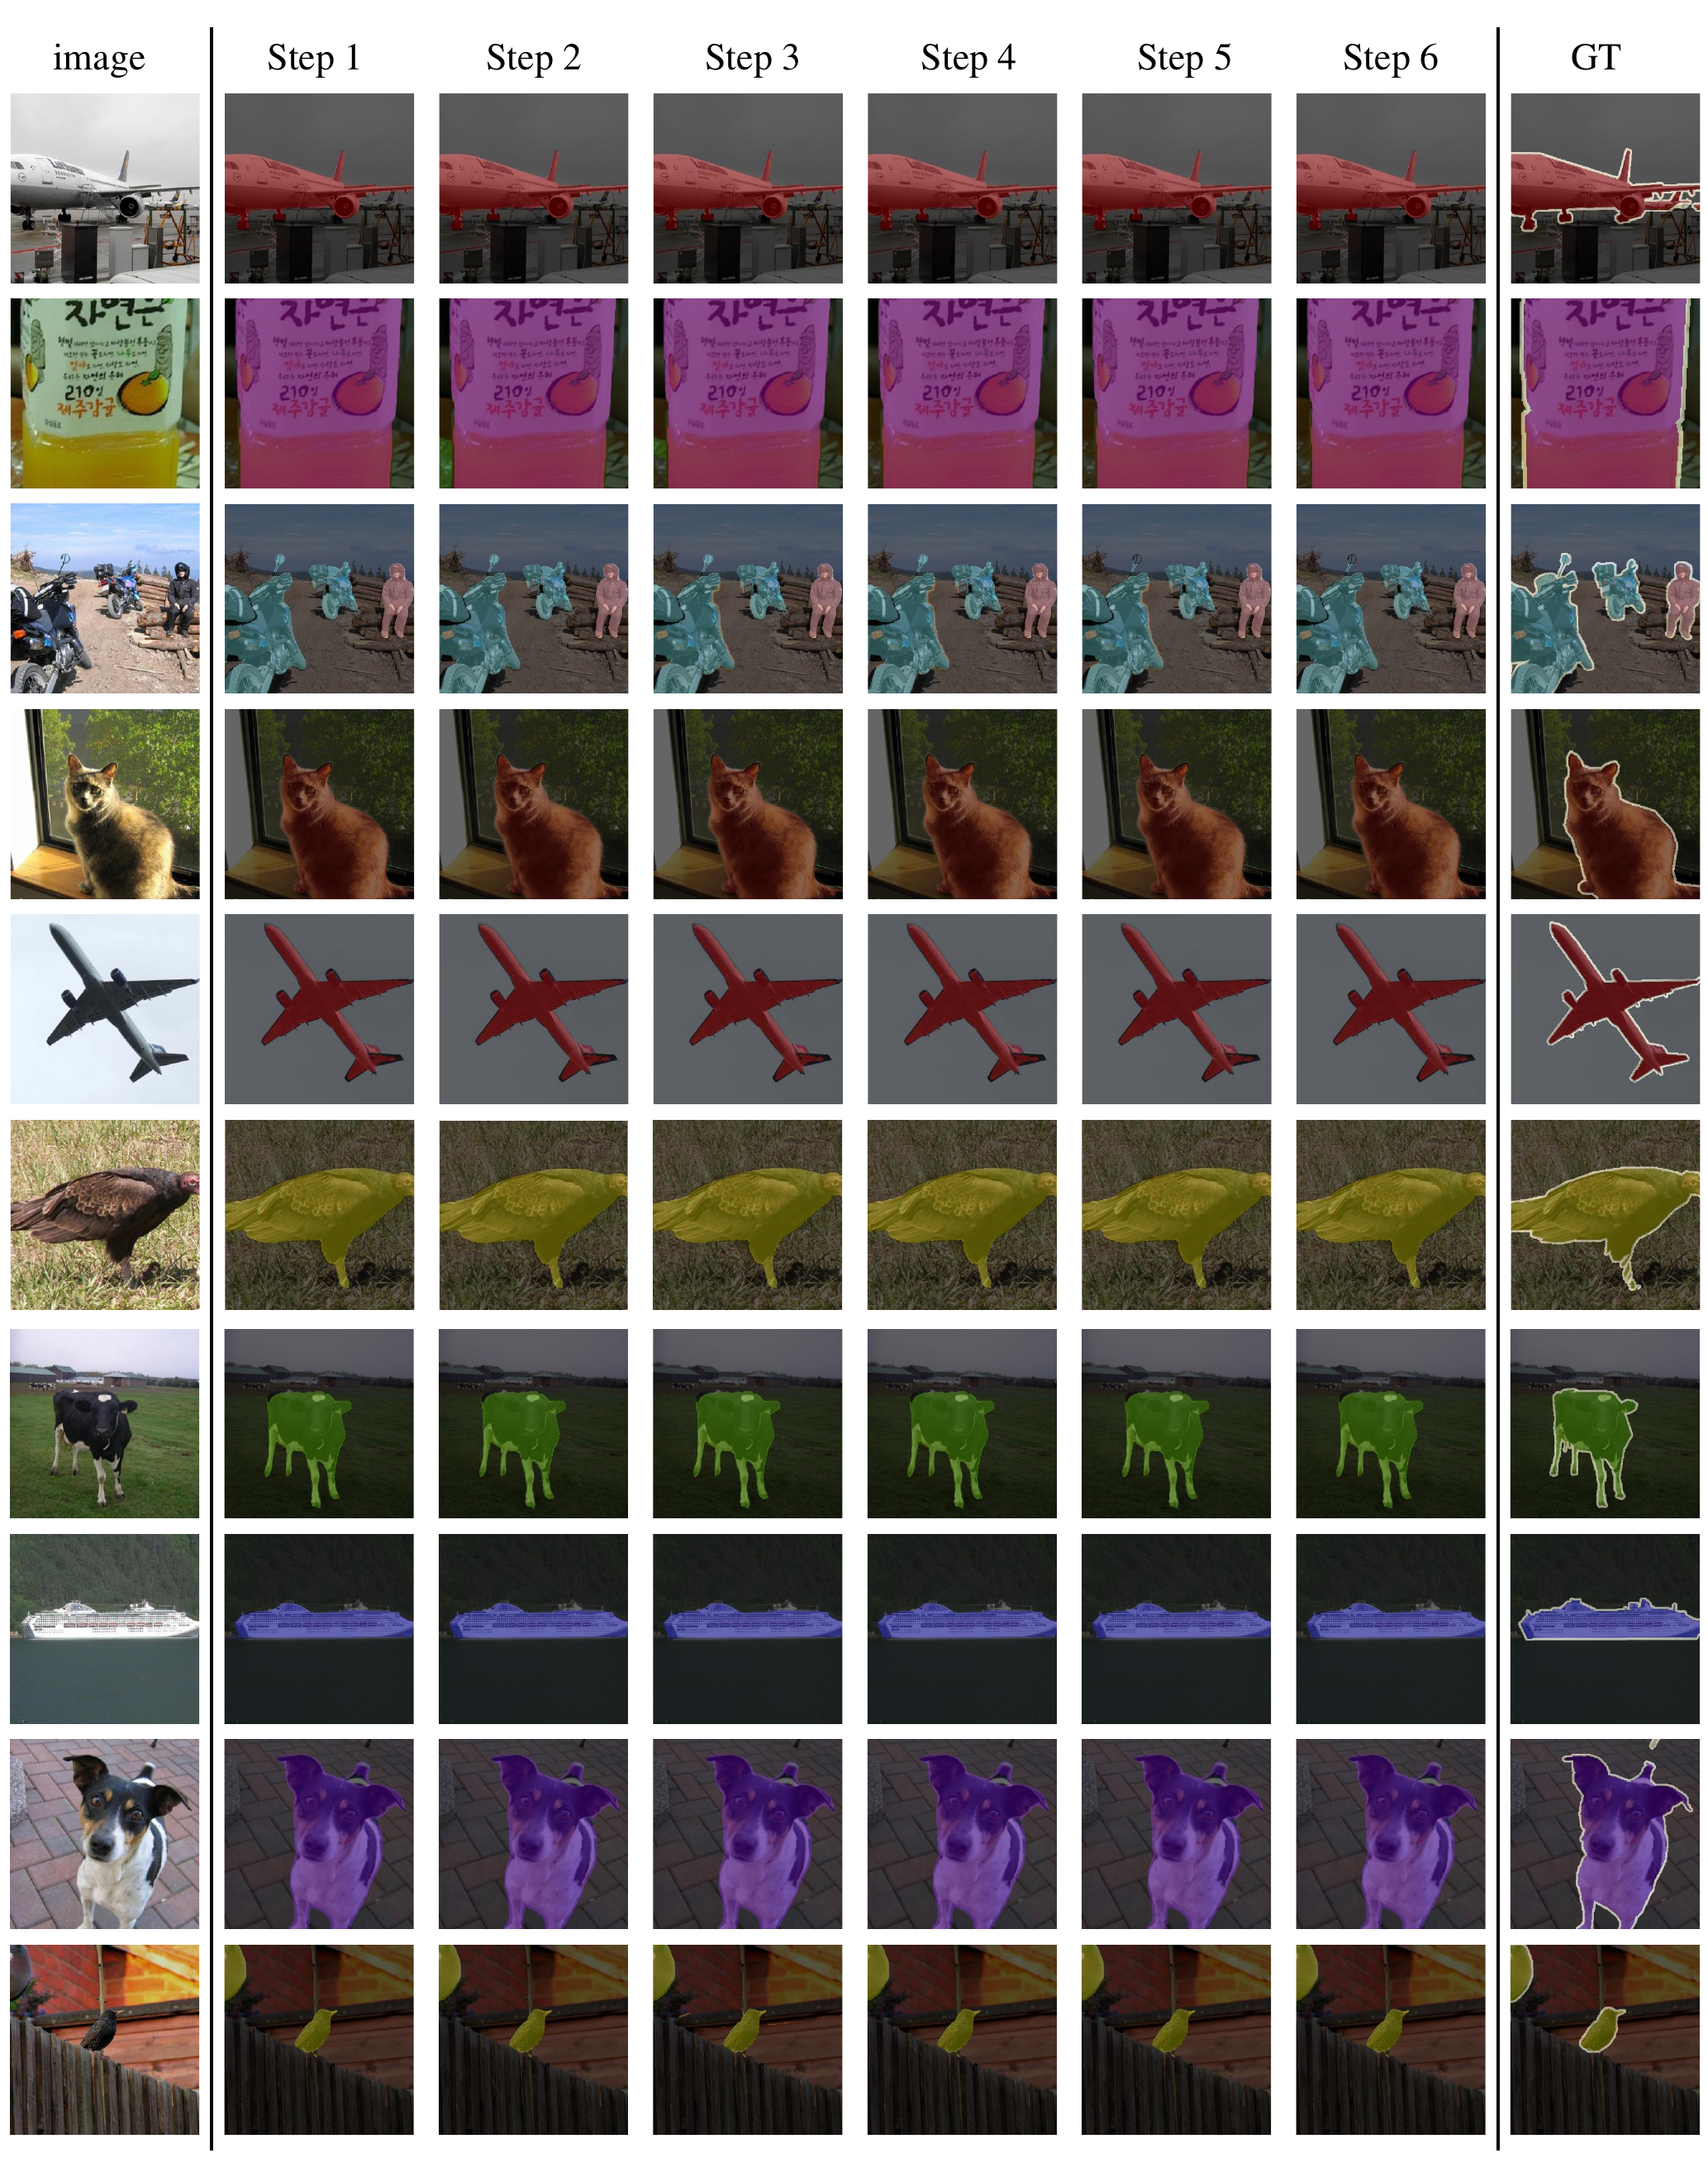}
}

\caption{{More qualitative analysis of CoinSeg. The white borderline is \textbf{ignore label} in Pascal VOC 2012 dataset.}}
% \vspace{-0.3cm}
\label{fig:quat_more2}
 \end{figure*}
